# Supplementary material for: When to Read Documents or QA History: On Unified and Selective Open-domain QA
Source: arXiv:2306.04176 source file (2023-06-07)
Supplement: Supplementary file 1 [file 7_appendix.tex]

\begin{appendices}

\section{Datasets and Implementation}\label{appendix_implementation}

We use the open-domain QA version of TriviaQA \cite{joshi2017triviaqa} and Natural Questions \cite{kwiatkowski2019natural}.
The details of the benchmarks are as follows:

\begin{itemize}[leftmargin=0.4cm]
\setlength\itemsep{2pt}
    \item \textbf{Natural Questions (NQ)} \cite{kwiatkowski2019natural} contains real user questions from Google search engine. We use training/dev/testing splits for open-domain question answering, consisting of 79K train, 8.7k dev, 3.6K test examples.
    \item \textbf{TriviaQA (TQA)} \cite{joshi2017triviaqa} is constructed from web-scraped trivia questions. We use TriviaQA open-domain training/dev/testing splits, consisting of 79K train, 8.8k dev, and 11K test examples.
\end{itemize}

We implement our models upon T5 with the size of 770M and 3B, and fine-tune them on NQ and TQA.
770M (or `Large') model and 3B (or `XL') model are trained from T5-large and T5-3B respectively.
When calculating the labels of sampling consistency, it requires a warm-up QA model. 
As the warm-up model, we train a base QA model until 1 epoch.
In our observation, early stopping at 1 epoch prevents from overfitting -- the consistency scores on train set converge to 1.
Our evaluation occurs at the end of each epoch during 5 epochs, and we select a best model on development set.

\section{Retrieval Implementation}\label{appendix_retrieval}

To retrieve the contexts ($\mathbf{d}$ and $\mathbf{k}$), we use the same off-the-shelf retrieval as used by baselines: FiD-KD \cite{izacard2020distilling} for Doc-QA, and RePAQ \cite{lewis2021paq} for QR.
For a collection of knowledge, we also use PAQ database for QA pairs \cite{lewis2021paq}, and Wikipedia for documents \cite{karpukhin2020dense}.

Table~\ref{retrieval} shows the accuracy of retrievals from documents and QA-pairs.
If a correct answer is included in the top-\textit{K} contexts, the retrieval is assumed to succeed.
While this measure calculated by naive string matching is commonly used in \cite{karpukhin2020dense,izacard2021leveraging,izacard2020distilling}, it is not perfect as false negative examples can be counted as true positive.

\input{tables/retrieval_result}

\section{Qualitative examples}
For the human-level insight, we provide qualitative examples from the actual prediction of our method.
We focus on demonstrating the effect of our proposed individual calibration measures -- answerability and sampling consistency.

%[Answerability - 3099, detect `distracted because unanswerable' case]
In Figure \ref{examples}, Example (a) contrasts the documents and QA pairs where the answerability is significantly lower for the former.
The retrieved documents do not contain the ground truth (\textit{`October 24, 2017'}),
hence the model infers the wrong answer from documents, while it predicts the correct answer from the successfully retrieved QA pairs.
Answerability reflects the estimated validity of retrieval, and thus helps us to distinguish the more reliable answer as in this example.

%[Consistency - 783 vs 102, detect `answerable but distracted' case]
Meanwhile, sampling consistency captures a more subtle interplay between the model and retrieved contexts.
In Figure \ref{examples} Example (b), both the retrieved documents and QA pairs contain the ground truth.
However, there is a distractive information in QA pairs (\textit{`Who played the bad guy in wonder woman?'}) as well, which misguides the QA model.
Even though the answer is misguided, we can see that the uncertainty is reflected in low sampling consistency for QA pairs, as opposed to the higher score for documents.

\begin{figure*}[t]
	\centering
	\includegraphics[width=162mm]{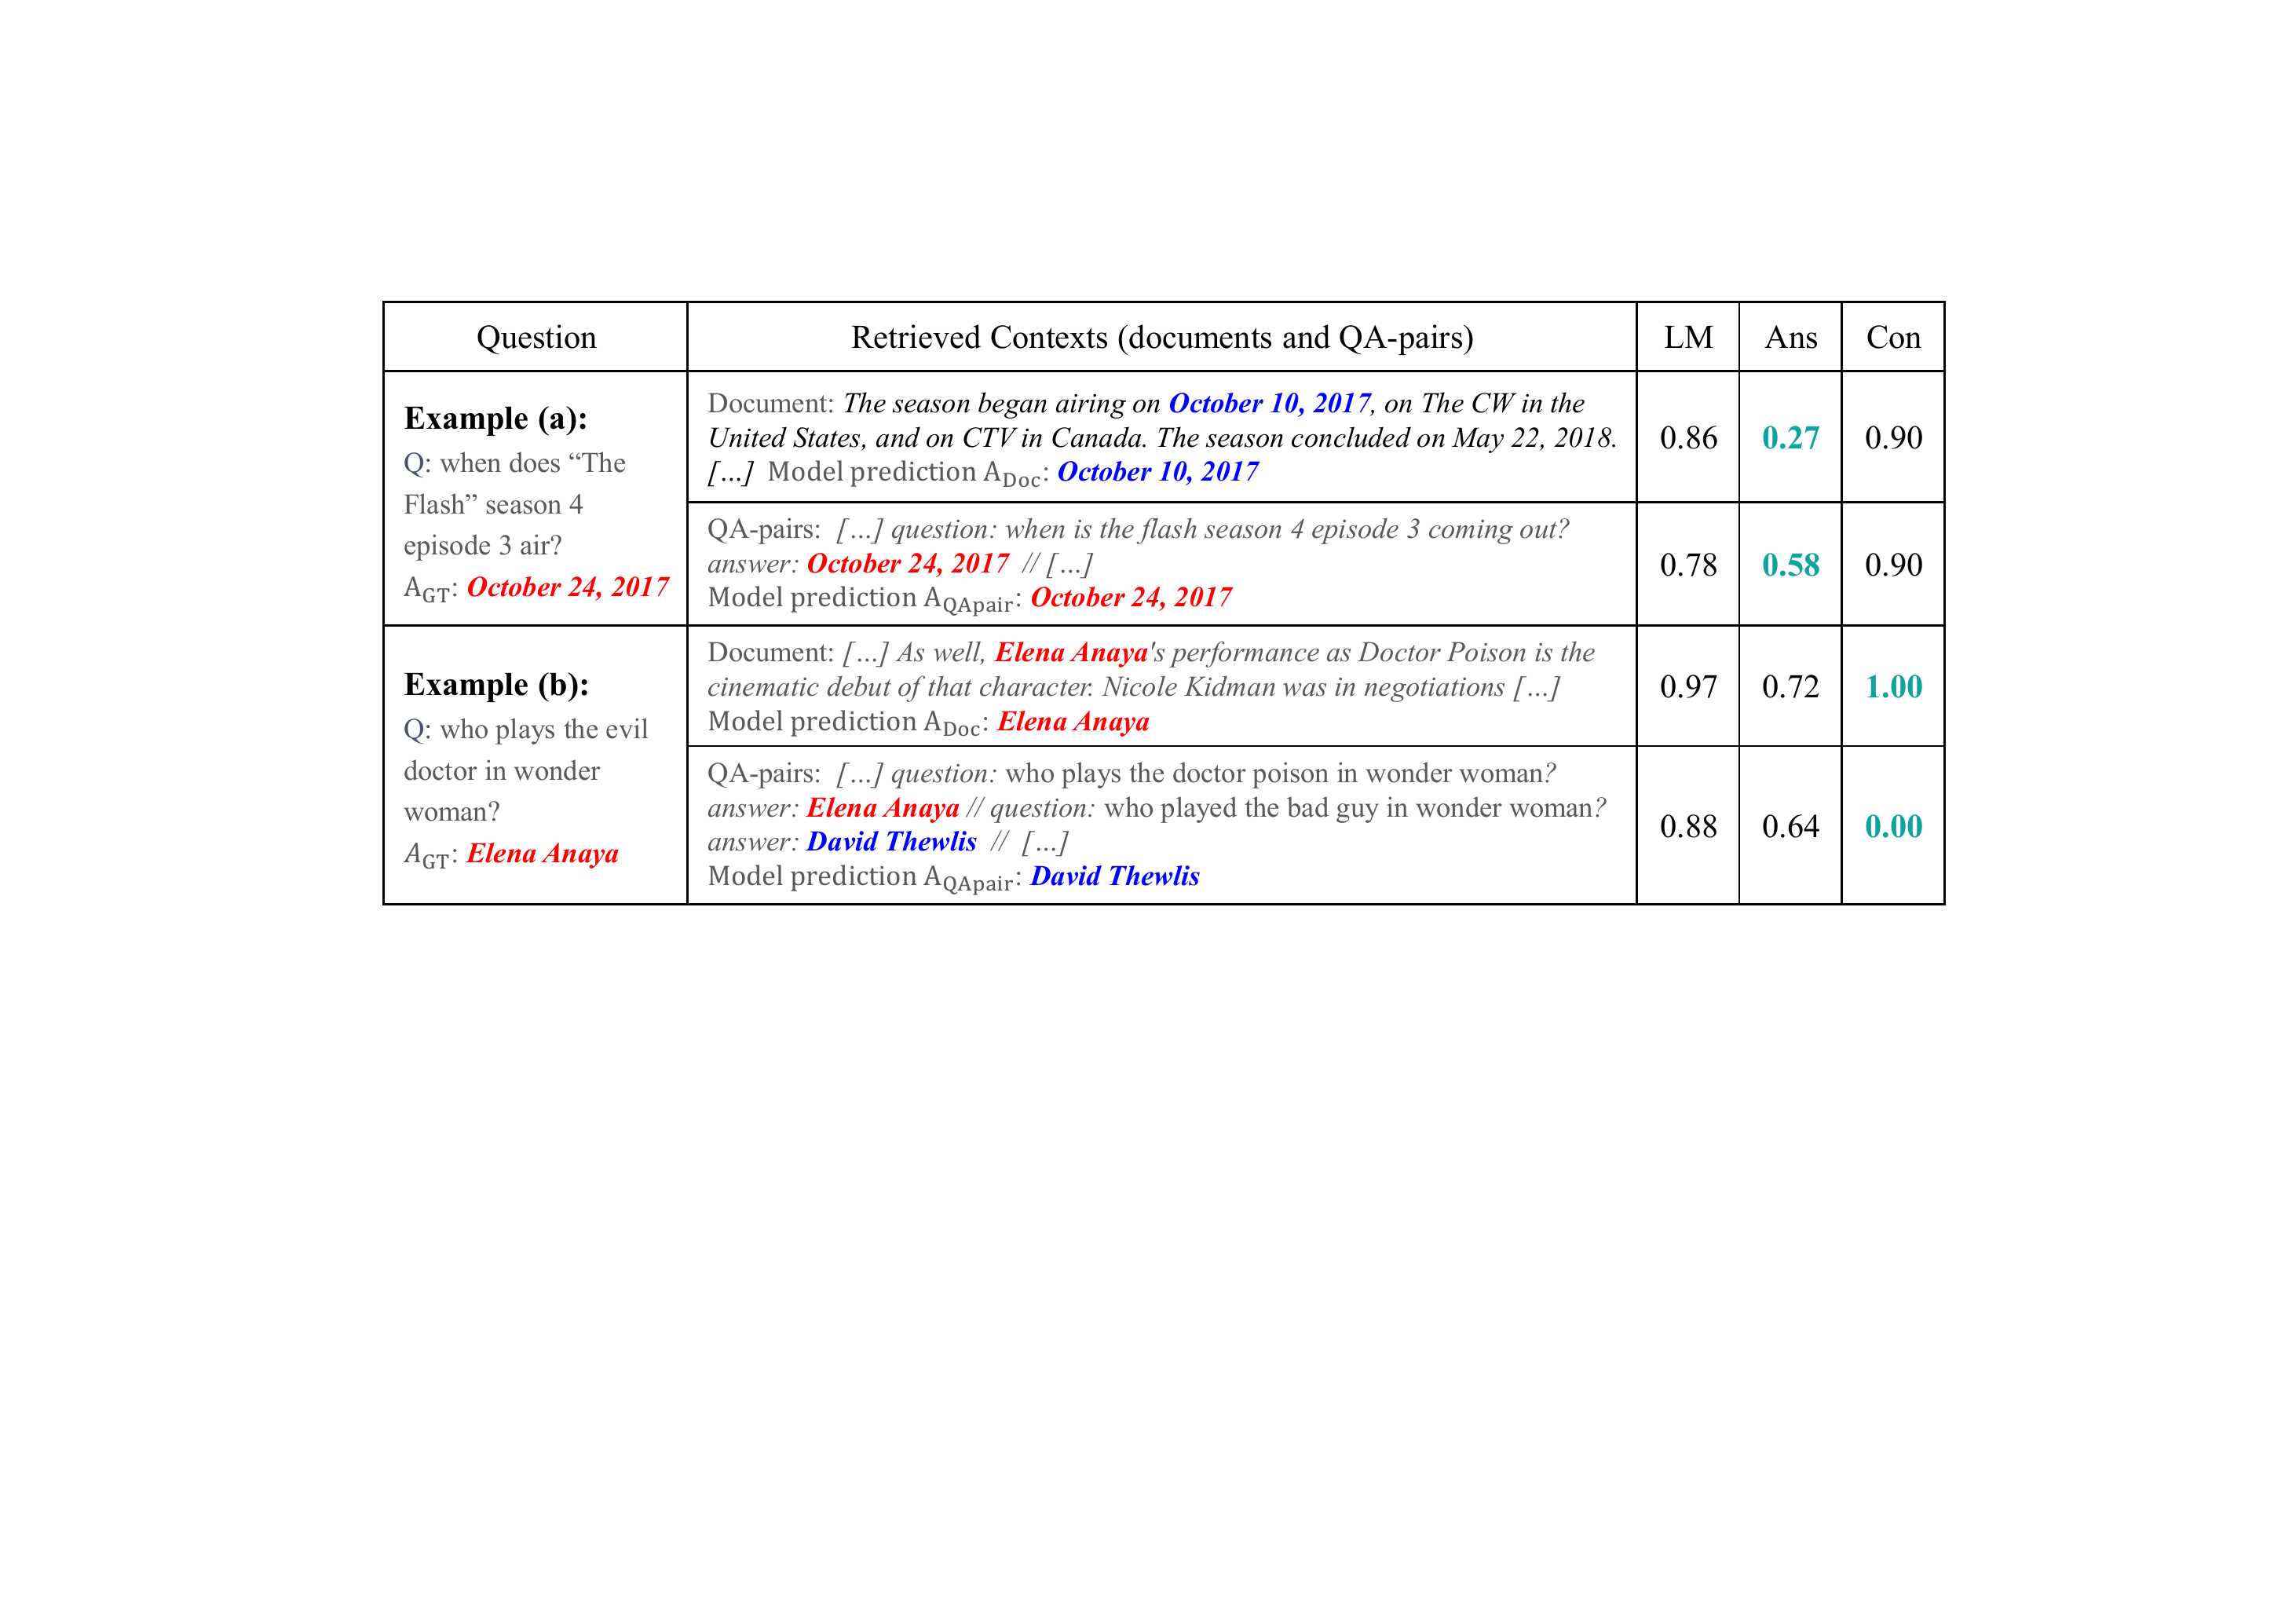}
	\caption{
Examples for (a) answerability and (b) sampling consistency. In (b), both documents and QA pairs have high answerability, but the QA pairs have lower sampling consistency due to the distraction. Correct answers are colored in red, while incorrect answers are in blue.
	}
	\label{examples}
\end{figure*}

\end{appendices}
